# Supplementary material for: Enhancing Maritime Situational Awareness through End-to-End Onboard Raw Data Analysis
Source: arXiv:2411.03403 source file (2024-11-05)
Supplement: Supplementary file 1 [file appendix_a.tex]

\appendix{}
\section{Appendix}\label{APPENDIX}

\begin{algorithm}[!h]
\caption{Create the Cost Matrix}\label{alg:alg_1}
\footnotesize
\begin{algorithmic}[1]
\State \textbf{Input:} BBox centers and AIS data
\State \textbf{Output:} Cost matrix $C$

\Procedure{Cost Matrix}{BBox centers, AIS data}
    \State $n \gets \text{number of bbox centers}$
    \State $m \gets \text{number of AIS points}$
    \State $C \gets$ Initialize a cost matrix of size $n \times m$

    \For{each bbox center $i$}
        \For{each AIS point $j$}
            \State $d_{\text{eucl}} \gets$ Calculate Euclidean distance between bbox center $i$ and AIS point $j$
            \If{there are two AIS coordinates for $j$}
                \State line $\gets$ Create a line from the two AIS coordinates
                \State $d_{\perp} \gets$ Calculate perpendicular distance from bbox center $i$ to the line
            \Else
                \State $d_{\perp} \gets d_{\text{eucl}}$
            \EndIf
            \State $s_j \gets$ Get navigational status for AIS point $j$
            \If{$s_j$ is 'Engaged in fishing'}
                \State $w_{\text{nav}} \gets 0.5$ \Comment{Prioritize fishing vessels}
            \Else
                \State $w_{\text{nav}} \gets 1.0$
            \EndIf
            \State $C_{ij} \gets w_{\text{nav}} \times (d_{\perp} + d_{\text{eucl}})$
        \EndFor
    \EndFor

    %\State Replace NaN or infinity values in $C$ with a large number (e.g., $\infty$)
    \State \Return $C$
\EndProcedure

\end{algorithmic}
\end{algorithm}

\begin{algorithm}[!h]
\caption{Hungarian Algorithm}\label{alg:alg_2}
\footnotesize
\begin{algorithmic}[1]
\State \textbf{Input:} Cost matrix $C$
\State \textbf{Output:} Optimal assignment of bbox centers to AIS points

\Procedure{Apply Hungarian Algorithm}{$C$}
    \State \textbf{Step 1: Solve the assignment problem}
    \State $(row\_ind, col\_ind) \gets$ Solve the assignment problem using the Hungarian algorithm on cost matrix $C$
    
    \State \textbf{Step 2: Process the matches}
    \For{each $i$ in $row\_ind$}
        \State $j \gets$ corresponding AIS index from $col\_ind$
        \If{$C_{ij}$ is not infinity}
            \State Store the matched bbox center $i$ with AIS point $j$
            \State Mark AIS point $j$ as used
        \EndIf
    \EndFor

    \State \textbf{Step 3: Handle unmatched AIS points}
    \For{each AIS point $j$ not used in the matches}
        \State Store the unmatched AIS point $j$
    \EndFor
    
    \State \textbf{Step 4: Ensure Unique Global Matches}
    \State Maintain a global dictionary of MMSI to bbox assignments
    \For{each global MMSI match}
        \If{MMSI already matched globally}
            \State Skip reassignment
        \Else
            \State Store the first valid match
        \EndIf
    \EndFor
    
    \State \textbf{Step 5: Return the result}
    \State \Return optimal assignment of bbox centers to AIS points and unmatched AIS point
\EndProcedure

\end{algorithmic}
\end{algorithm}
